# Supplementary material for: Social Conjuring: Multi-User Runtime Collaboration with AI in Building Virtual 3D Worlds
Source: arXiv:2410.00274 source file (2024-10-02)
Supplement: Supplementary file 1 [file dataset-distribution-table.tex]

\begin{table}[ht]
\centering
\begin{tabular}{|c|c|}
\hline
\textbf{Spatial Relationship} & \textbf{Count} \\ \hline
Above  & 164  \\ \hline
Behind & 111  \\ \hline
Below  & 161  \\ \hline
Front  & 111  \\ \hline
Left   & 146  \\ \hline
Right  & 147  \\ \hline
\end{tabular}
\caption{Distribution of Spatial Relationships}
\label{tab:spatial-relationships}
\end{table}
